# Supplementary material for: Ultrafast optical ranging using microresonator soliton frequency combs
Source: arXiv:1707.05969 ancillary file (2017-07-20)
Supplement: Supplementary file 1 [file SupplementaryMaterials.pdf]

# Ultrafast optical ranging using microresonator soliton frequency combs - Supplementary Information -


Philipp Trocha[1,×], Denis Ganin[1,×], Maxim Karpov[2,×], Martin H. P. Pfeiffer[2], Arne Kordts[2], Jonas Krockenberger[1], Stefan Wolf[1], Pablo Marin-Palomo[1], Claudius Weimann[1,4], Sebastian Randel[1,3], Wolfgang Freude[1,3], Tobias J. Kippenberg[2,*], Christian Koos[1,3,*]

[1] *Institute of Photonics and Quantum Electronics (IPQ), Karlsruhe Institute of Technology (KIT), 76131 Karlsruhe, Germany*
[2] *École Polytechnique Fédérale de Lausanne (EPFL), 1015 Lausanne, Switzerland*
[3] *Institute of Microstructure Technology (IMT), Karlsruhe Institute of Technology (KIT), 76131 Karlsruhe, Germany*
[4] *Now with: Corporate Research and Technology, Carl Zeiss AG, Oberkochen, Germany*
[×] *These authors contributed equally to this work*
[*] christian.koos@kit.edu, tobias.kippenberg@epfl.ch


# 1 Mathematical description of distance metrology scheme

The LIDAR method applied in our experiments is based on a multi-heterodyne phase measurement of the lines of an optical frequency comb that travels to a target and back. In this section, we give a rigorous mathematical description of the measurement scheme, see Figure 1 for a graphical illustration. Complex analytical signals $\underline{E}(\mathrm{t})$ are used to describe the time-domain electric fields, with the real part of the analytical signal representing the physically relevant field, $E(\mathrm{t}) = \Re\{\underline{E}(\mathrm{t})\}$. A signal comb (index S, orange) with frequencies $\omega_{\mathrm{S},\mu} = \omega_{\mathrm{S},0} + \mu\omega_{\mathrm{S,r}}$ is split in two parts at a beam splitter (BS). The first part of the comb leaves the setup, is reflected by the target, coupled back into the system after traversing a total free-space distance 2*d*, and finally routed towards a measurement photodetector (PD). The second part of the signal comb is directly guided towards the reference photodetector. Both parts of the signal comb are superimposed with two parts of another comb, acting as a local oscillator (index LO, blue) with frequencies $\omega_{\mathrm{LO},\nu} = \omega_{\mathrm{LO},0} + \nu\omega_{\mathrm{LO,r}}$. At a certain optical distance $L_\mathrm{S}$ and $L_\mathrm{LO}$ along the path of the respective comb, the complex electric fields of the signal and the LO comb are given by

$$\begin{aligned}\underline{E}_\mathrm{S}(L_\mathrm{S},t) &= \sum_\mu \underline{E}_{\mathrm{S},\mu}(L_\mathrm{S},t) = \sum_\mu \hat{\underline{E}}_{\mathrm{S},\mu} \exp\left[\mathrm{j}\left(\omega_{\mathrm{S},\mu}t - \omega_{\mathrm{S},\mu}/c\cdot L_\mathrm{S}\right)\right]\\ \underline{E}_\mathrm{LO}(L_\mathrm{LO},t) &= \sum_\nu \underline{E}_{\mathrm{LO},\nu}(L_\mathrm{LO},t) = \sum_\nu \hat{\underline{E}}_{\mathrm{LO},\nu} \exp\left[\mathrm{j}\left(\omega_{\mathrm{LO},\nu}t - \omega_{\mathrm{LO},\nu}/c\cdot L_\mathrm{LO}\right)\right]\end{aligned} \tag{1}$$

In these definitions, $\hat{\underline{E}}_{\mathrm{S},\mu}, \hat{\underline{E}}_{\mathrm{LO},\nu}$, denote the complex initial amplitudes at the output of the respective comb source, $\omega_{\mathrm{S},0}, \omega_{\mathrm{LO},0}$ are the associated center frequencies, and $\omega_{\mathrm{S,r}}, \omega_{\mathrm{LO,r}}$ denote the repetition rates. Upon reaching the measurement photodetector, the distance traveled by the signal comb from its source amounts to $L_\mathrm{S} = L_\mathrm{S,meas} + 2d$, comprising the free-space distance *d*, and a total setup internal optical distance $L_\mathrm{S,meas}$. The distance towards the reference photodetector is given in the same manner by $L_\mathrm{S} = L_\mathrm{S,ref}$. Equivalently, the optical path lengths from the LO comb source to the respective photodetector are defined as $L_\mathrm{LO} = L_\mathrm{LO,meas}$ and $L_\mathrm{LO} = L_\mathrm{LO,ref}$. The superposition of the signal and the LO comb (violet) on the measurement photodetector with sensitivity $S$ and effective detection area *A* leads to a photocurrent

$$i_\mathrm{meas}(t) = \frac{SA}{Z_0}\left\langle\left(\Re\left\{\underline{E}_\mathrm{S}\left(L_\mathrm{S,meas}+2d,t\right) + \underline{E}_\mathrm{LO}\left(L_\mathrm{LO,meas},t\right)\right\}\right)^2\right\rangle. \tag{2}$$

Here, $Z_0$ denotes the free-space impedance and the brackets $\langle\cdot\rangle$ denote averaging over several optical cycles, which eliminates any expressions oscillating at the optical sum frequencies. In addition, DC terms are cancelled in practice by using balanced photodetectors. The remaining AC-part of the photocurrent of the measurement detector consists of discrete tones, one of which is indicated as green sinusoidal oscillation in ,

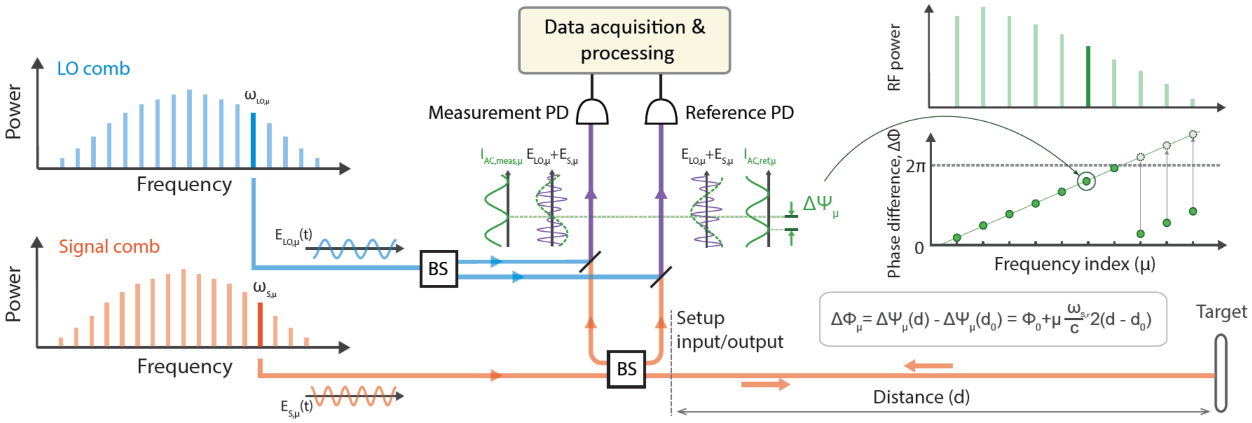


**Figure 1: Frequency-comb based multi-heterodyne interferometry.** Measurement principle: The signal comb (orange) and the LO comb (blue) consist of discrete tones at frequencies $\omega_{\mathrm{S},\mu}$ and $\omega_{\mathrm{LO},\mu}$. The superposition of these comb lines on the measurement PD and the reference PD leads to a multitude of beat notes in the RF spectrum of the photocurrent (green) at frequencies $\Delta\omega_\mu = \left|\omega_{\mathrm{LO},\mu} - \omega_{\mathrm{S},\mu}\right|$, which can be separated by a Fourier transform. The phases $\Phi_{\mathrm{meas},\mu}$ of these beat notes depend on the target distance d and can be extracted by comparison to the phases $\Phi_{\mathrm{ref},\mu}$ of the corresponding beat notes on the reference PD. The distance is finally obtained by estimating the slope of the phase differences as a function of frequency index $\mu$, see lower right-hand side.

$$
\begin{aligned}
i_{\mathrm{AC,meas}}(t) &= \frac{SA}{Z_0}\cdot\Re\left\{\underline{E}_S^*\left(L_{\mathrm{S,meas}}+2d,t\right)\underline{E}_{\mathrm{LO}}\left(L_{\mathrm{LO,meas}},t\right)\right\} \\
&= \frac{SA}{Z_0}\cdot\Re\left\{\begin{array}{l}\sum\limits_\mu\sum\limits_\nu \hat{\underline{E}}^*_{S,\mu}\hat{\underline{E}}_{\mathrm{LO},\nu}\exp\left(\mathrm{j}\left(\omega_{\mathrm{LO},0}-\omega_{\mathrm{S},0}+(\nu-\mu)\omega_{\mathrm{S,r}}+\nu\left(\omega_{\mathrm{LO,r}}-\omega_{\mathrm{S,r}}\right)\right)t\right) \\ \cdot\exp\left(\underbrace{\mathrm{j}\frac{\omega_{\mathrm{S},\mu}}{c}\left(L_{\mathrm{S,meas}}+2d\right)}_{=-\Psi_{\mathrm{meas},\mu}}-\mathrm{j}\frac{\omega_{\mathrm{LO},\nu}}{c}L_{\mathrm{LO,meas}}\right)\end{array}\right\}.
\end{aligned}
\tag{3}
$$

Note that this equation implicitly contains the optical phase $\Psi_{\mathrm{meas},\mu}$ defined in Eq. (1) of main text, labeled by an underbrace in the last line. The distance of interest $2d$ can be extracted from the phase of the various beat notes, which are visible in the photocurrent. However, as can be seen from Eq. (3), these phases also depend on the phases of the complex products $\hat{\underline{E}}^*_{S,\mu}\hat{\underline{E}}_{\mathrm{LO},\nu}$. To extract only the phases that are relevant to the distance, an independent reference measurement is required, which is obtained by superimposing separate parts of the same frequency combs on the separate reference photodetector, see also . The AC-part of the photocurrent $i_{\mathrm{AC,ref}}$ of the reference detector is derived in an analogous way to Eq. (3), by replacing "meas" by "ref" in the subscripts:

$$
\begin{aligned}
i_{\mathrm{AC,ref}}(t) &= \frac{SA}{Z_0}\cdot 2\Re\left\{\underline{E}_{\mathrm{S}}^*\left(L_{\mathrm{S,ref}},t\right)\underline{E}_{\mathrm{LO}}\left(L_{\mathrm{LO,ref}},t\right)\right\} \\
&= \frac{SA}{Z_0}\cdot 2\Re\left\{\begin{array}{l}\sum\limits_\mu\sum\limits_\nu \hat{\underline{E}}^*_{S,\mu}\hat{\underline{E}}_{\mathrm{LO},\nu}\exp\left(\mathrm{j}\left(\omega_{\mathrm{LO},0}-\omega_{\mathrm{S},0}+(\nu-\mu)\omega_{\mathrm{S,r}}+\nu\left(\omega_{\mathrm{LO,r}}-\omega_{\mathrm{S,r}}\right)\right)t\right) \\ \cdot\exp\left(\underbrace{\mathrm{j}\frac{\omega_{S,\mu}}{c}L_{\mathrm{S,ref}}}_{=-\Psi_{\mathrm{ref},\mu}}-\mathrm{j}\frac{\omega_{\mathrm{LO},\nu}}{c}L_{\mathrm{LO,ref}}\right)\end{array}\right\}.
\end{aligned}
\tag{4}
$$

In contrast to Eq. (3), the external measurement distance $2d$ does not appear in the reference path lengths. Note that the underbraced expression in the last line of Eq. implicitly contains the optical phases $\Psi_{\mathrm{ref},\mu}$ defined in Eq. (1) of the main manuscript.

The repetition rate detuning $\Delta\omega_r = \left|\omega_{\text{LO,r}} - \omega_{\text{S,r}}\right|$ amounts to roughly $\Delta\omega_r = 2\pi\cdot 100$ MHz and is small compared to the line spacing of roughly $\omega_{\text{S,r}} = 2\pi\cdot 100$ GHz. In theory, the photocurrent spectrum shows beat signals at distinct intermediate frequencies

$$\omega_{\nu,\mu} = \left|\omega_{\text{LO},0} - \omega_{\text{S},0} + (\nu-\mu)\,\omega_{\text{S,r}} + \nu\,\Delta\omega_{\text{r}}\right| \tag{5}$$

However, only a subset of these lines can actually be acquired by the photodetector and the subsequent analog-to-digital converter (ADC). For the frequency combs deployed in our experiments, the analog bandwidth *B* of the ADC used to record the signals amounts to 32 GHz and is clearly smaller than the half the 100 GHz line spacing of the frequency combs, $B < \omega_{\text{S,r}}/2 \approx \omega_{\text{LO,r}}/2$ . Moreover, the number of comb lines is limited such that $\nu\Delta\omega_{\text{r}} < \omega_{\text{S,r}}/2 \approx \omega_{\text{LO,r}}/2$ for all comb line indices $\nu$ . As a consequence, for a given LO comb line $\nu$ , only the beat note with the corresponding signal comb line of same index $\nu = \mu$ is visible in the photocurrent. These beat notes are found at distinct frequencies $\Delta\omega_\mu = \left|\Delta\omega_0 + \mu\,\Delta\omega_{\text{r}}\right|$ with $\Delta\omega_0 = \left|\omega_{\text{LO},0} - \omega_{\text{S},0}\right|$ being the difference of the center frequencies of the two combs. The beat notes, shown in the upper right of  as a function of frequency index $\mu$, can be identified and extracted by means of a discrete Fourier transform (DFT) of the time-domain photocurrents recorded by the oscilloscope.

The phases $\Phi_{\text{meas},\mu}$ and $\Phi_{\text{ref},\mu}$ of these beat notes in the photocurrents $i_{\text{AC,meas},\mu}$ and $i_{\text{AC,ref},\mu}$ depend on the various distances $L_{\text{S,meas}}, L_{\text{LO,meas}}, L_{\text{S,ref}}, L_{\text{LO,ref}}$ that the signal comb and the reference comb have traveled from the respective source to the respective detector. Exact expressions for these phases can be derived from Eq. (3) and (4) by setting $\nu = \mu$ and by considering the complex amplitude of the various harmonic oscillations,

$$\begin{aligned}
\Phi_{\text{meas,}\mu}(d) &= \arg\left\{\underline{\hat{E}}^{*}_{\text{S},\mu}\,\underline{\hat{E}}_{\text{LO},\mu}\exp\left(\text{j}\frac{\omega_{S,\mu}}{c}\left(L_{\text{S,meas}}+2d\right) - \text{j}\frac{\omega_{\text{LO},\mu}}{c}L_{\text{LO,meas}}\right)\right\} \\
&= \frac{\omega_{S,0}+\mu\omega_{\text{S,r}}}{c}\left(L_{\text{S,meas}} - L_{\text{LO,meas}} + 2d\right) - \frac{\Delta\omega_0+\mu\Delta\omega_{\text{r}}}{c}L_{\text{LO,meas}} + \arg\left\{\underline{\hat{E}}^{*}_{\text{S},\mu}\,\underline{\hat{E}}_{\text{LO},\mu}\right\} \\
&= 2\pi\left(L_{\text{S,meas}} - L_{\text{LO,meas}} + 2d\right)\Lambda_\mu^{-1} + 2\pi\left(L_{\text{S,meas}} - L_{\text{LO,meas}} + 2d\right)\lambda_{\text{S},0}^{-1} \\
&\quad - \frac{\Delta\omega_0+\mu\Delta\omega_{\text{r}}}{c}L_{\text{LO,meas}} + \arg\left\{\underline{\hat{E}}^{*}_{\text{S},\mu}\,\underline{\hat{E}}_{\text{LO},\mu}\right\},
\end{aligned} \tag{6}$$

$$\begin{aligned}
\Phi_{\text{ref,}\mu} &= \arg\left\{\underline{\hat{E}}_{\text{S},\mu}\,\underline{\hat{E}}^{*}_{\text{LO},\mu}\exp\left(\text{j}\frac{\omega_{S,\mu}}{c}L_{\text{S,ref}} - \text{j}\frac{\omega_{\text{LO},\mu}}{c}L_{\text{LO,ref}}\right)\right\} \\
&= \frac{\omega_{S,0}+\mu\omega_{\text{S,r}}}{c}\left(L_{\text{S,ref}} - L_{\text{LO,ref}}\right) - \frac{\Delta\omega_0+\mu\Delta\omega_{\text{r}}}{c}L_{\text{LO,ref}} + \arg\left\{\underline{\hat{E}}_{\text{S},\mu}\,\underline{\hat{E}}^{*}_{\text{LO},\mu}\right\} \\
&= 2\pi\left(L_{\text{S,ref}} - L_{\text{LO,ref}}\right)\Lambda_\mu^{-1} + 2\pi\left(L_{\text{S,ref}} - L_{\text{LO,ref}}\right)\lambda_{\text{S},0}^{-1} \\
&\quad - \frac{\Delta\omega_0+\mu\Delta\omega_{\text{r}}}{c}L_{\text{LO,ref}} + \arg\left\{\underline{\hat{E}}_{\text{S},\mu}\,\underline{\hat{E}}^{*}_{\text{LO},\mu}\right\}.
\end{aligned} \tag{7}$$

In these relations, the function $\arg\{\underline{z}\}$ denotes the phase angle of a complex number $\underline{z}$ . The last lines of Eq. (6) and (7) contain the so-called synthetic wavelength $\Lambda_\mu = c\left(\mu\,\omega_{\text{S,r}}/2\pi\right)^{-1}$ and show the relation to classical interferometry with a single optical wavelength $\lambda$ , where the phase shift $\varphi$ experienced by an optical signal after propagation over the optical path length $L$ is determined by $\varphi = 2\pi L\lambda^{-1}$.

As expected, the phases of the beat notes in the reference and the measurement photocurrent depend on the initial phases $\arg\left\{\underline{\hat{E}}^{*}_{\text{S},\mu}\,\underline{\hat{E}}_{\text{LO},\mu}\right\}$ of the corresponding optical comb tones. Mathematically, these initial phases can be eliminated by calculating the differences of the phases observed from the reference and the measurement detector,

$$\delta\Phi_\mu(d) = \Phi_{\text{meas},\mu}(d) - \Phi_{\text{ref},\mu}$$
$$= \frac{\omega_{S,0} + \mu\omega_{\text{S,r}}}{c}\left(L_{\text{S,meas}} + 2d - L_{\text{LO,meas}} - L_{\text{S,ref}} + L_{\text{LO,ref}}\right) - \frac{\Delta\omega_0 + \mu\Delta\omega_{\text{r}}}{c}\left(L_{\text{LO,meas}} - L_{\text{LO,ref}}\right). \tag{8}$$

Subtracting the values $\Delta\Phi_\mu(d_0)$ from a calibration measurement for a specific distance $d_0$, we can further eliminate all expressions that depend on the internal optical path lengths $L_{\text{S,meas}}$, $L_{\text{S,ref}}$, $L_{\text{LO,meas}}$, $L_{\text{LO,ref}}$,

$$\Delta\Phi_\mu(d,d_0) = \delta\Phi_\mu(d) - \delta\Phi_\mu(d_0) = \frac{\omega_{\text{S},0}}{c}\times 2(d-d_0) + \mu\frac{\omega_{\text{S,r}}}{c}\times 2(d-d_0). \tag{9}$$

This equation shows that there is a linear relation between the phase difference $\Delta\Phi_\mu$ and the frequency index $\mu$, see also  on the right, in which phase differences that would exceed $2\pi$ have been unwrapped. Equation (9) can be reshaped to elaborate the relationship of the distance $(d-d_0)$ and slope of $\Delta\Phi_\mu$ vs $\mu$:

$$\Delta\Phi_\mu(d,d_0) = \Delta\Phi_0(d,d_0) + \mu\frac{\omega_{\text{S,r}}}{c}\times 2(d-d_0) \tag{10}$$

Equation (10) is used to determine the distance  by extracting the slope of the linear relationship between $\Delta\Phi_\mu$ and $\mu$. In the experiments, this slope is obtained by extracting the phases of the various photocurrents by means of a Fourier transform, by unwrapping them, and by fitting a straight line to the measured values of $\Delta\Phi_\mu$ vs. $\mu$. The associated fit error can be used as a measure of the quality of the raw data and allows us to define an independent criterion for evaluating the reliability of certain measurements.

It is important to note that the calibration measurement for a specific distance $d_0$ is only valid as long as the internal path lengths $L_{\text{S,meas}}, L_{\text{S,ref}}, L_{\text{LO,meas}}, L_{\text{LO,ref}}$ do not change. In our setup, however, the associated fiber links are subject to environmental influences such as temperature drift of optical fibers, which can lead to drifts of tens of micrometers per second and per meter of fiber [1], [2]. For measurements at highest precision over an extended set of data points, it is hence important to perform the calibration measurement simultaneously with the actual measurement to minimize the associated errors and to allow separating measurement errors that are intrinsic to the measurement technique from drift of the optical setup. In technical implementations of measurement systems, the impact of fiber drift can be eliminated by minimizing fiber lengths or by introducing dedicated reference mirrors into the system, which are used for permanent calibration.

# 2 Distance sweep over ambiguity interval and calibration measurements

To demonstrate the ability of our system to accurately measure distances over the full ambiguity interval, we use a high-precision feedback-stabilized positioning stage (Physik Instrumente, M511.HD) having an accuracy of better than 50 nm [3]. This experiment took an extended amount of time for signal acquisition and evaluation at each data point such that fiber drift [1], [2] during the measurement must be taken into account, see previous section as well as e and the associated explanations in the main paper. To separate measurement errors that are intrinsic to our technique from drift of the optical setup, the distance measurement is switched between the movable target mirror and a static calibration mirror in intervals of approximately 300 µs, which is fast enough to eliminate even drift of the approximately 5 to 10 m long fiber paths that were deployed in our setup. Fast switching between the mirrors is accomplished by the experimental setup shown in Figure 2a. The measurement beam is split by a beam splitter (BS) and then routed to two mirrors. One mirror is in a fixed position (calibration mirror, CM) and another one is mounted to movable stage (target mirror, TM). A rotating chopper wheel (RCW) blocks always one of the two beam paths, such that the distance to the calibration and the measurement mirror can be independently determined in quick succession. Figure 2b shows an exemplary measurement: Two distinct levels are visible, indicated by orange points. Between the levels, the determined phase values are noisy due to a superposition of optical signals received from both mirrors. This leads to unreliable distance information, indicated by large fit errors of the linear phase characteristics according to Eq. (2) of the main text, based on which the erroneous points (blue) were discarded from

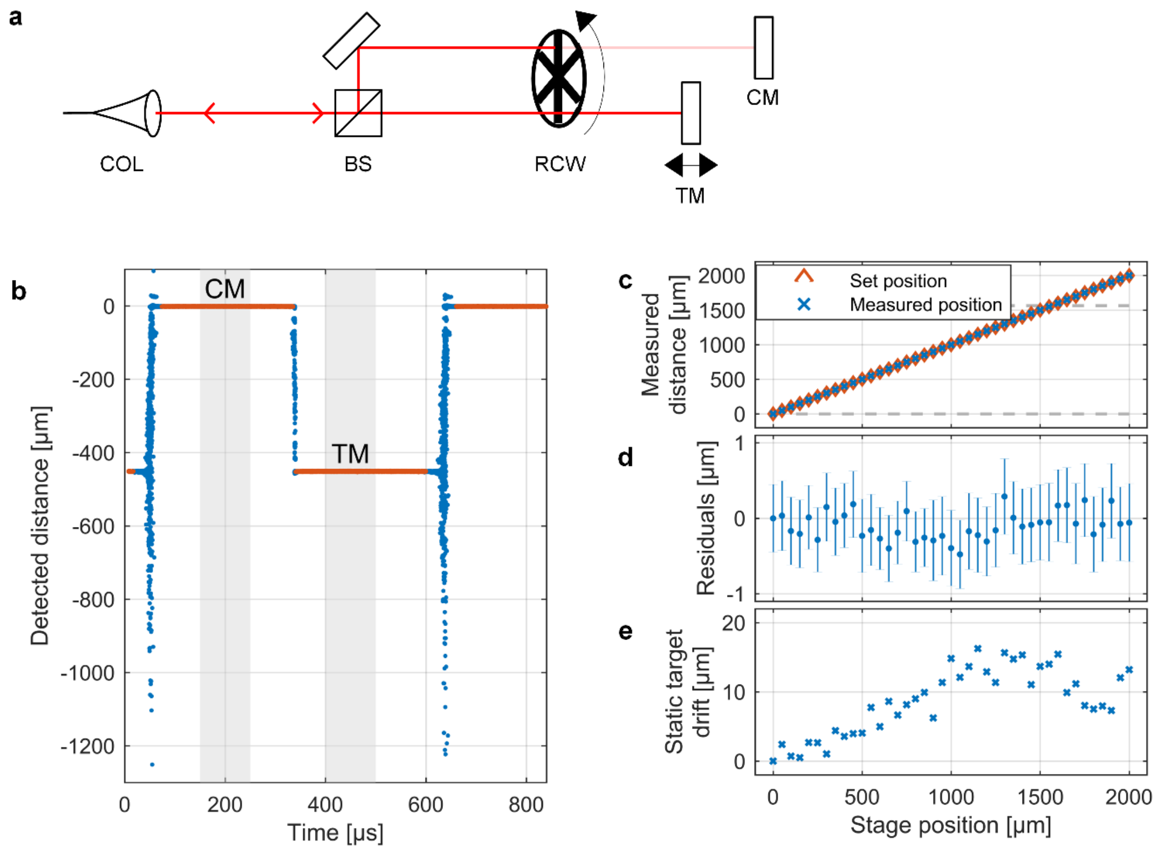


**Figure 2: Distance sweep over the ambiguity interval of the system**. **(a)** Experimental setup: The measurement beam leaves the setup via a fiber collimator (COL), is split by a beam splitter (BS) and sent to two mirrors, one fixed serving as a calibration mirror (CM) and the other as a movable target mirror (TM) on a feedback-stabilized positioning stage. A rotating chopper wheel (RCW) ensures that only one signal from either of these mirrors is coupled back into the system at a certain instant in time. This allows independent measurements of the TM and the fixed CM distance. **(b)** Measurement showing the distance profile over time. The measured distances to the calibration and the target mirror are indicated in orange, separated by noisy transitions (blue) during which signals were received from both mirrors. This leads to unreliable distance information, indicated by large fit errors of the linear phase characteristics according to Eq. (2) of the main text, based on which the erroneous points (blue) were discarded from further analysis. Gray shaded areas show sections, over which the respective distance and standard deviation is evaluated **(c)** Distance sweep of the target mirror over a full ambiguity interval. Blue crosses denote distances measured by our system, whereas orange diamonds indicate the distance set by the stage. A manual "unwrapping" of the measured distances was performed beyond the ambiguity interval (grey dashed lines). **(d)** Residual deviations ("residuals") between the measured and the set distance. The residuals are of the same order of magnitude as the 50 nm positioning accuracy of the positioning stage, as specified by the manufacturer. Error bars indicate the standard deviation. **(e)** Drift of the distance measured to the CM over time. Drift magnitudes 20 µm are in line with expectations, given fiber lengths between 5 m and 10 m in our setup and typical drifts of tens of micrometers per second and per meter of fiber [1], [2].

further analysis. In our measurements, the distance close to zero is related to the calibration mirror. The difference between the two levels is computed by evaluating the data at the highest possible acquisition rate of 97.7 MHz, by performing an average over the gray shaded sections with a duration of 100 µs, and by subtracting the two averaged distances afterwards. In a first measurement, we determine the distance difference between target and calibration mirror for the first arbitrary position of the target mirror and use it as a zero-position for all subsequent measurements. The target mirror is then stepped in increments of 50 µm, and the differences between target and calibration mirror distances are measured. The results are shown in Figure 2c, where the set and measured positions are compared. In the plot, we have performed a manual "unwrapping" of the measured distances beyond the ambiguity distance of our system.

Figure 2d shows the residual differences ("residuals") between the measured position and the distance set by the stage. Note that these residuals are of the same order of magnitude as the 50 nm positioning accuracy of the positioning stage specified

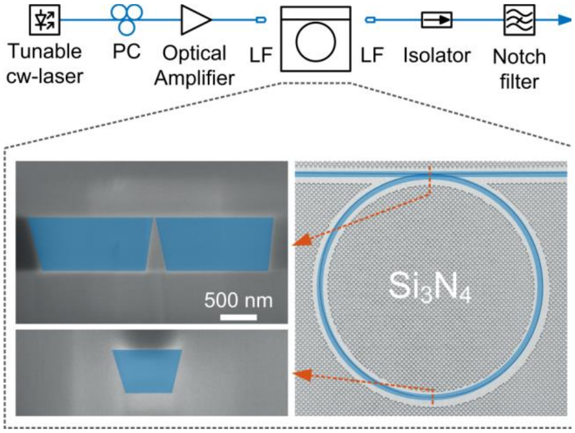


**Figure 3: Principle of soliton frequency comb generation in high-Q silicon nitride ($Si_3N_4$) microresonators.** The integrated photonic microresonator is pumped by a tunable continuous-wave (cw) laser, which is amplified by an erbium-doped fiber amplifier (Optical Amplifier). Lensed fibers (LF) are used to couple light to the chip. A fiber polarization controller (PC) is used to optimize the power in the waveguide. After the microresonator, a notch filter suppresses remaining pump light and an isolator prevents back-propagation of backscattered pump light. The insets show scanning electron microscopy images of a $Si_3N_4$ microresonator with a radius of 240 µm. Right inset, top view. The checker-board pattern results from the photonic Damascene fabrication process [6]. Left insets, cross-sections of the resonator waveguide (indicated by the dashed red arrows; dimensions, 0.8 µm × 1.65 µm) at the coupling point (top) and at the tapered section (bottom; dimensions, 0.8 µm × 0.6 µm). The tapered section is used for suppressing higher-order modes [10] while preserving a high optical quality factor ($Q \approx 10^6$). (Figure adapted from [9])

by the manufacturer [3] and that they do not show any cyclic error. The error bars shown in Figure 2d denote the standard deviation of all measurements taken within the gray shaded sections at a certain position of the target mirror. Figure 2e shows the absolute distances to the calibration mirror that were acquired during the measurement. Neighboring data points were taken at intervals of approximately 45 s, dictated by the settling time of the stage and by the data acquisition speed. The plot reveals a clear drift of the order of 15 µm, which we attribute to thermal drift of the fiber lengths [1], [2]. This drift might also be one of the main causes for the residuals observed in Figure 2d.

# 3 Kerr Soliton frequency comb generation in $Si_3N_4$ microresonators

Our work relies on integrated silicon-nitride ($Si_3N_4$) microresonators [4], [5] for generation of dissipative Kerr-soliton (DKS) frequency combs, see . The $Si_3N_4$ platform is chosen because of its low optical losses and its compatibility with large-scale silicon-based processing [4]. The microresonators have a waveguide height of 800 nm to achieve anomalous group velocity dispersion and are fabricated using the photonic Damascene process [6]. Neighboring resonances are spaced by approximately 96.5 GHz and have intrinsic quality (Q) factors exceeding $10^6$. DKS combs are obtained by sweeping the pump laser through the resonance from a blue-detuned wavelength to a predefined red-detuned wavelength [5], [7]. This leads initially to the generation of modulation-instability Kerr combs followed by DKS states once the resonance is crossed. Importantly, once a multiple-soliton comb state is generated, the transition to a single-soliton state can be accomplished in a reliable and deterministic manner [8] by adjusting the laser frequency. The soliton comb states are remarkably stable for many hours in a laboratory environment, which is key to the distance measurements presented.

The distances extracted from a linear fit of the phases according to Eq. (10) still depend on the line spacing $\omega_{\mathrm{S,r}}$ of the signal comb. For high measurement precision, this line spacing must be continuously tracked. This is accomplished by determining the line spacing $\omega_{\mathrm{LO,r}}$ of the LO comb and then deriving $\omega_{S,r} = \omega_{\mathrm{LO,r}} + \Delta\omega_{\mathrm{r}}$ from the known spacing $\Delta\omega_{\mathrm{r}}$ of the baseband beat notes. To measure the LO line spacing $\omega_{\mathrm{LO,r}}$, a part of the LO pump laser light is modulated by a Mach-Zehnder modulator (MZM) at a known frequency $\omega_{\mathrm{mod}}$, such that strong third-order sidebands are generated. This signal is overlapped with the LO comb, and the line spacing $\omega_{\mathrm{LO,r}}$ is derived by monitoring the corresponding RF beat notes of the side bands and the nearest comb line.

# 4 Measurement accuracy

The measurement accuracy of our technique depends on both the number of comb lines and the optical bandwidth that is covered by these combs. In this section, we derive a relationship between the standard deviation $\sigma_d$ of the measured distance $d$, the number $N$ of comb lines, the optical bandwidth $\Omega_{\mathrm{S}} = N \cdot \omega_{S,r}$ of the signal comb, and the standard deviation

$\sigma_\phi$ associated with measuring the optical phases. According to Eq. (10), the relation between the ideal phase values $\Delta\Phi_\mu$ and the distance $\left(d-d_0\right)$ is given by

$$\Delta\Phi_\mu = \Delta\Phi_0 + \mu\frac{\omega_{\mathrm{S,r}}}{c}2\left(d-d_0\right), \tag{11}$$

where $\omega_{S,r}$ is the signal comb repetition rate and *c* the speed of light in vacuum. For extracting the distance $\left(d-d_0\right)$ from measured phase values, we estimate the slope $D$ of $\Delta\Phi_\mu$ with respect to the frequency index $\mu$,

$$D = \frac{\omega_{\mathrm{S,r}}}{c}2\left(d-d_0\right). \tag{12}$$

In the experiment, the estimation of *D* relies on actually measured phase values $\Delta\hat{\Phi}_\mu$ that are distorted by noise, leading to small random deviations $\phi_{\mathrm{n},\mu}$ from the ideally expected phases $\Delta\Phi_\mu$ according to Eq. (11).

$$\Delta\hat{\Phi}_\mu = \Delta\Phi_0 + \mu D + \phi_{\mathrm{n},\mu} \ . \tag{13}$$

These random deviations $\phi_{\mathrm{n},\mu}$ will lead to stochastic errors of the extracted slope *D*. In the following, we assume that all noise contributions $\phi_{\mathrm{n},\mu}$ feature the same stochastic distribution and that they are statistically independent as well as mean-free. The standard deviation is denoted as $\sigma_{\phi,\mu} = \sigma_\phi \, \forall \mu$. The confidence interval of a slope *D* estimated from a linear regression of noisy ordinate data is proportional to the variance $\sigma_D^2$ of the slope, which, according to [11], can be expressed as

$$\sigma_D^2 = \frac{\sigma_\phi^2}{\sum_{\mu=1}^{N}\left(\mu-\bar{\mu}\right)^2} \ . \tag{14}$$

In this relation, $\bar{\mu}$ denotes the mean of all abscissa values used for the regression. In the denominator of Eq. (14), the frequency index $\mu$ has been chosen to vary between 1 and $N$ to simplify the subsequent derivation. Note that, by substituting the index, any other range of integers can be chosen, e.g., between $-(N-1)/2$ and $+(N-1)/2$ for odd integers N, without changing the validity of the final results of this analysis. For the range chosen here, the mean value $\bar{\mu}$ is given by

$$\bar{\mu} = \frac{N\left(N+1\right)}{2}. \tag{15}$$

The denominator of Eq. (14) can thus be simplified to

$$\sum_{\mu=1}^{N}\left(\mu-\bar{\mu}\right)^2 = \frac{N(N^2-1)}{12} \approx \frac{N^3}{12} \quad \text{for } N >> 1 \, . \tag{16}$$

Substituting Eq. (16) into Eq. (14), we obtain

$$\sigma_D^2 = \sigma_\phi^2 \frac{12}{N^3}. \tag{17}$$

With that, we can estimate the standard deviation $\sigma_d$ of the measured distance using Eq. (12)

$$\sigma_d = \frac{c}{2\omega_{S,r}} \cdot \sigma_D = \sqrt{\frac{3}{N^3}}\frac{c}{\omega_{S,r}}\sigma_\phi = \sqrt{\frac{3}{N}}\frac{c}{\Omega_{\mathrm{S}}}\sigma_\phi, \tag{18}$$

where $\Omega_{\mathrm{S}} = N\omega_{\mathrm{S,r}}$ denotes overall optical bandwidth of the comb. For high-speed sampling, the number *N* of optical lines is limited since a minimum observation time $T_{\min} = 1/\Delta f_r \geq N / f_{\mathrm{ADC}}$ is required to spectrally resolve the various baseband beat notes by a Fourier transformation, where $f_{\mathrm{ADC}}$ is the maximum analog bandwidth that the analogue-to-digital converter (ADC) can acquire, see Section "Vision and Concept" of the main paper. For a fixed total number *N* of optical lines, the only option that remains for improving the measurement accuracy is thus to increase the overall optical bandwidth $\Omega = N\omega_{\mathrm{S,r}}$ of the comb, which requires a comb source that provides a large free spectral range $\omega_{\mathrm{S,r}}$. DKS combs stand out due to a unique combination of optical bandwidth and large FSR. They feature comparatively few optical lines and are therefore perfectly suited for simultaneously achieving high acquisition rate and high measurement accuracy.

# 5 References


[1] C. Weimann, F. Hoeller, Y. Schleitzer, C. A. Diez, B. Spruck, W. Freude, Y. Boeck, and C. Koos, “Measurement of Length and Position with Frequency Combs,” *J. Phys. Conf. Ser.*, vol. 605, p. 12030, 2015.

[2] G. B. Hocker, “Fiber-optic sensing of pressure and temperature,” *Appl. Opt.*, vol. 18, no. 9, p. 1445, 1979.

[3] Physics Instruments, “MP84E User Manual M-511.HD Ulta-High-Resolution Positioner,” 2008.

[4] J. S. Levy, A. Gondarenko, M. a. Foster, A. C. Turner-Foster, A. L. Gaeta, and M. Lipson, “CMOS-compatible multiple-wavelength oscillator for on-chip optical interconnects,” *Nat. Photonics*, vol. 4, no. 1, pp. 37–40, 2010.

[5] V. Brasch, T. Herr, M. Geiselmann, G. Lihachev, M. H. P. Pfeiffer, M. L. Gorodetsky, and T. J. Kippenberg, “Photonic chip-based optical frequency comb using soliton Cherenkov radiation,” *Science (80-. ).*, vol. 351, no. 6271, pp. 357–360, 2016.

[6] M. H. P. Pfeiffer, A. Kordts, V. Brasch, M. Zervas, M. Geiselmann, J. D. Jost, and T. J. Kippenberg, “Photonic Damascene process for integrated high-Q microresonator based nonlinear photonics,” *Optica*, vol. 3, no. 1, pp. 20–25, 2016.

[7] T. Herr, V. Brasch, J. D. Jost, C. Y. Wang, N. M. Kondratiev, M. L. Gorodetsky, and T. J. Kippenberg, “Soliton mode-locking in optical microresonators,” *Nat. Photonics*, vol. 8, no. 2, pp. 145–152, 2013.

[8] M. Karpov, H. Guo, E. Lucas, A. Kordts, M. H. P. Pfeiffer, G. Lichachev, V. E. Lobanov, M. L. Gorodetsky, and T. J. Kippenberg, “Universal dynamics and controlled switching of dissipative Kerr solitons in optical microresonators,” *Nat. Phys.*, vol. 13, pp. 94–102, 2017.

[9] P. Marin-Palomo, J. N. Kemal, M. Karpov, A. Kordts, J. Pfeifle, M. H. P. Pfeiffer, P. Trocha, S. Wolf, V. Brasch, M. H. Anderson, R. Rosenberger, K. Vijayan, W. Freude, T. J. Kippenberg, and C. Koos, “Microresonator solitons for massively parallel coherent optical communications,” *Nat. Publ. Gr.*, vol. 546, no. 7657, pp. 274–279, 2016.

[10] A. Kordts, M. Pfeiffer, H. Guo, V. Brasch, and T. J. Kippenberg, “Higher order mode suppression in high-Q anomalous dispersion SiN microresonators for temporal dissipative Kerr soliton formation,” *Opt. Lett.*, vol. 41, no. 3, pp. 452–455, 2015.

[11] D. C. Montgomery, E. A. Peck, and G. G. Vining, *Introduction to Linear Regression Analysis* (Wiley, 2013).
